# Supplementary material for: PyRQA -- Conducting Recurrence Quantification Analysis on Very Long Time Series Efficiently
Source: arXiv:2402.16853 source file (2024-01-18)
Supplement: Supplementary file 1 [file appendix.tex]

\section{Source Code - Climatological Data.}
\label{real_world_example}

\lstinputlisting[language=Python, 
		      basicstyle=\footnotesize, 
		      frame=single]{real_world_example.py}
		    
\section{Source Code - Synthetic Data.}
\label{synthetic_example}

\lstinputlisting[language=Python,  
		      basicstyle=\footnotesize, 
		      frame=single]{synthetic_example.py}
